# Supplementary material for: Nonlinear Biochemical Signal Processing via Noise Propagation
Source: arXiv:1309.2588 source file (2013-09-10)
Supplement: Supplementary file 1 [file sensitivity-supp.pdf]

# Supplementary Information: Nonlinear Biochemical Signal Processing via Noise Propagation

Kyung Hyuk Kim*[1], Hong Qian[1,2] , Herbert M. Sauro[2]

[1] Department of Bioengineering, University of Washington, William H. Foege Building, Box 355061, Seattle, WA 98195, U.S.A.
[2] Department of Applied Mathematics, University of Washington, Lewis Hall, Box 353925, Seattle, WA 98195, U.S.A.

Email: Kyung Hyuk Kim - kkim@uw.edu; Hong Qian - hqian@u.washington.edu; Herbert M Sauro - hsauro@uw.edu;

*Corresponding author

## S1 Derivation of Eqs. (B3) and (B4)

From the master equation (A1) by multiplying $S_k$ (molecule number) and summing over all possible states, we obtain

$$\begin{aligned}\frac{d\langle S_k\rangle_t}{dt} &= \sum_S S_k \sum_{j=1}^{R}\Big[\Big(\prod_{i=1}^{m} E^{-N_{R_{ij}}}\Big)-1\Big]V_j P \\ &= \sum_S\sum_{j=1}^{n}\Big[(S_k-N_{R_{kj}})\Big(\prod_{i=1}^{m}E^{-N_{R_{ij}}}\Big)V_jP - S_kV_jP\Big] + \sum_S\sum_{j=1}^{n}N_{R_{kj}}\Big(\prod_{i=1}^{m}E^{-N_{R_{ij}}}\Big)V_jP \\ &= \sum_S\sum_{j=1}^{n}\Big[\Big(\prod_{i=1}^{m}E^{-N_{R_{ij}}}\Big)S_kV_jP - S_kV_jP\Big] + \sum_S\sum_{j=1}^{n}N_{R_{kj}}V_jP, \end{aligned} \tag{S1}$$

where $E^{-N_{R_{ij}}}$ is a raising-lowering operator that changes molecule numbers by $-N_{R_{ij}}$ such that $E^{-N_{R_{ij}}}f(\boldsymbol{S}) = f(\{S_{ij}-N_{R_{ij}}\})$. The first term on the right hand side of Eq (S1) vanishes since the first summation is performed over all the possible states and the sum value does not depend on the existence of the raising-lowering operator. We now switch this number representation to concentration by replacing $\boldsymbol{S}\to\Omega\boldsymbol{s}$ and $\boldsymbol{V}\to\Omega\boldsymbol{v}$ in Eq. (S1), and finally, we obtain the following equation:

$$\frac{d\langle \boldsymbol{s}\rangle}{dt} = \boldsymbol{N}_R\langle \boldsymbol{v}(\boldsymbol{s},\boldsymbol{p})\rangle_t. \tag{S2}$$

This equation will be used to derive Eq. (B3).

We introduce a number covariance matrix $\boldsymbol{\Sigma}_t$ defined as:

$$\Sigma^t_{ij} \equiv \Big\langle (S_i-\langle S_i\rangle_t)(S_j-\langle S_j\rangle_t)\Big\rangle_t.$$

From the master equation by multiplying $(S_k - \langle S_k\rangle_t)(S_l - \langle S_l\rangle_t)$ and summing over all possible states, we obtain

$$\begin{aligned}
\frac{d\Sigma^t_{kl}}{dt} &= \sum_S (S_k - \langle S_k\rangle_t)(S_l - \langle S_l\rangle_t)\sum_{j=1}^{n}\Big[\Big(\prod_{i=1}^{m} E^{-N_{R_{ij}}}\Big) - 1\Big]V_j P \\
&= \sum_S \sum_{j=1}^{n}\Big[\Big(\prod_{i=1}^{m} E^{-N_{R_{ij}}}\Big)(S_k - \langle S_k\rangle_t + N_{R_{kj}})(S_l - \langle S_l\rangle_t + N_{R_{lj}}) - (S_k - \langle S_k\rangle_t)(S_l - \langle S_l\rangle_t)\Big]V_j P \\
&= \sum_{j=1}^{n}\Big\langle (S_k - \langle S_k\rangle_t + N_{R_{kj}})(S_l - \langle S_l\rangle_t + N_{R_{lj}})V_j - (S_k - \langle S_k\rangle_t)(S_l - \langle S_l\rangle_t)V_j\Big\rangle_t \\
&= \sum_{j=1}^{n}\Big\langle (S_k - \langle S_k\rangle_t)N_{R_{lj}}V_j + V_j N_{R_{kj}}(S_l - \langle S_l\rangle_t) + N_{R_{kj}}N_{R_{lj}}V_j\Big\rangle_t \\
&= \Big\langle\Big[(\boldsymbol{S} - \langle\boldsymbol{S}\rangle_t)^T(\boldsymbol{N}_R\boldsymbol{V})^T + (\boldsymbol{N}_R\boldsymbol{V})(\boldsymbol{S} - \langle\boldsymbol{S}\rangle_t) + \boldsymbol{N}_R\boldsymbol{\Lambda}'\boldsymbol{N}_R^T\Big]\Big\rangle_t\Big|_{kl},
\end{aligned}$$

where $\Lambda'_{ij} \equiv V_i\delta_{ij}$. By switching the number representation to concentrationrepresentation ($\boldsymbol{S} \to \Omega\boldsymbol{s}$, $\boldsymbol{V} \to \Omega\boldsymbol{v}$, $\boldsymbol{\Sigma} \to \Omega^2\boldsymbol{\sigma}, \boldsymbol{\Lambda}' \to \Omega\boldsymbol{\Lambda}$), we derive the following equation.

$$\frac{d\boldsymbol{\sigma}_t}{dt} = \Big\langle (\boldsymbol{N}_R\boldsymbol{v})(\boldsymbol{s} - \langle\boldsymbol{s}\rangle_t) + (\boldsymbol{s} - \langle\boldsymbol{s}\rangle_t)^T(\boldsymbol{N}_R\boldsymbol{v})^T + \frac{\boldsymbol{D}}{\Omega}\Big\rangle_t. \tag{S3}$$

This equation will be used to derive Eq. (B4). We note that Eqs. (S2) and (S3) were derived without any approximation from the master equation.

From Eqs. (S2) and (S3), we can obtain equations (B3) and (B4), by using the Taylor expansion of the reaction rate $\boldsymbol{v}$ with respect to the mean concentration levels and by neglecting the third and higher moments. These approximations become reasonable when the system shows single-peak and sufficiently narrow probability distributions near the stationary state. Under the approximation, Eq. (S2) becomes

$$\frac{d\langle\boldsymbol{s}\rangle_t}{dt} = \boldsymbol{N}_R\Big\langle \boldsymbol{v}(\langle\boldsymbol{s}\rangle_t, \boldsymbol{p})\rangle_t + \sum_{i=1}^{m_0}\frac{\partial\boldsymbol{v}}{\partial s_i}\Big|_{\boldsymbol{s}=\langle\boldsymbol{s}\rangle_t}(s_i - \langle s_i\rangle_t) + \frac{1}{2}\sum_{i,j=1}^{m}\frac{\partial^2\boldsymbol{v}}{\partial s_i\partial s_j}\Big|_{\boldsymbol{s}=\langle\boldsymbol{s}\rangle_t}(s_i - \langle s_i\rangle_t)(s_j - \langle s_j\rangle_t)\Big\rangle_t.$$

The second term on the right hand side vanishes because $\langle s_i - \langle s_i\rangle_t\rangle_t = \langle s_i\rangle_t - \langle s_i\rangle_t = 0$. Therefore, Eq. (B3) is derived.

By applying the Taylor expansion, the first term on the right hand side of Eq. (S3) becomes, after neglecting the third and higher moments:

$$\big\langle(\boldsymbol{N}_R\boldsymbol{v})(\boldsymbol{s} - \langle\boldsymbol{s}\rangle_t)\big\rangle_t = \boldsymbol{N}_R\boldsymbol{v}(\langle\boldsymbol{s}\rangle_t)\big\langle(\boldsymbol{s} - \langle\boldsymbol{s}\rangle_t)\big\rangle_t + \boldsymbol{J}\boldsymbol{\sigma}_t = \boldsymbol{J}\boldsymbol{\sigma}_t.$$

By using the same procedure, the second term on the right hand side of Eq. (S3) becomes $\boldsymbol{\sigma}_t^T\boldsymbol{J}^T$ and the third term becomes:

$$\langle\Lambda_{ij}\rangle_t = \delta_{ij}\langle v_i\rangle_t = \delta_{ij}\Big[v_i(\langle\boldsymbol{s}\rangle_t) + \frac{\partial v_i}{\partial\boldsymbol{s}}\Big|_{\boldsymbol{s}=\langle\boldsymbol{s}\rangle_t}\big\langle(\boldsymbol{s} - \langle\boldsymbol{s}\rangle_t)\big\rangle_t\Big],$$

where the second term vanishes. Therefore, by combining all these results, we derive Eq. (B4).

## S2 Stochastic focusing compensation in inhibitory regulation

In this section we investigate stochastic focusing compensation further for inhibition reaction steps with different dissociation constants. The inhibition reaction is modeled by

$$v(s) = \frac{c}{K_M + s}.$$

Figure S1 shows stochastic focusing (SF) and stochastic de-focusing (SD) appeared strongly when $K_M \simeq 0.1$ nM and thus the elasticity changed dramatically due to noise. As $K_M$ increases, SF-SD becomes weaker and the changes in the elasticity becomes less.

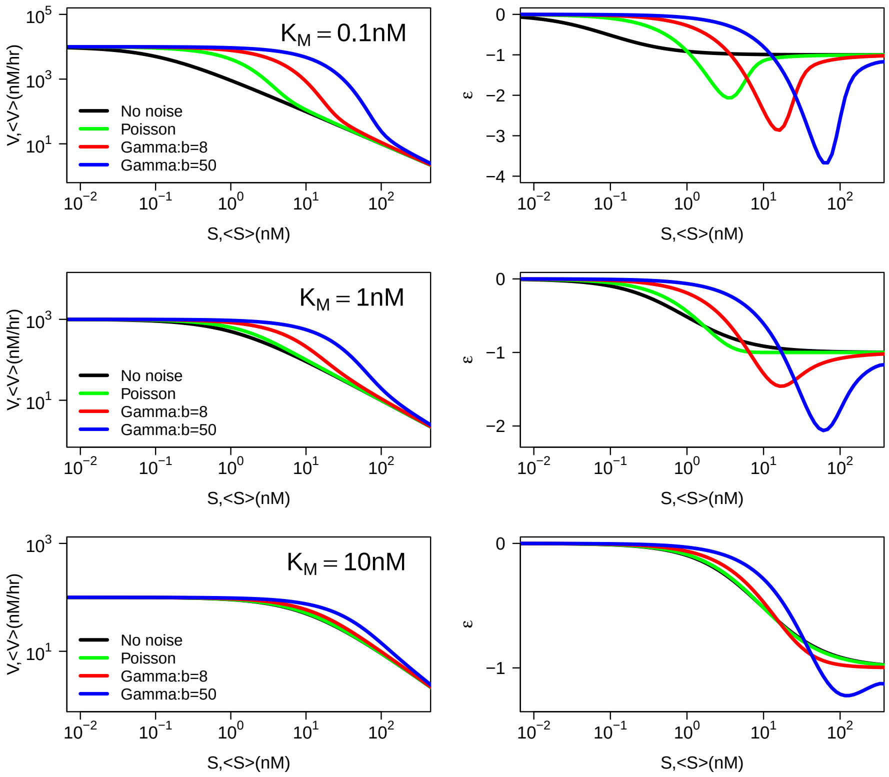


**Figure S1.** Stochastic focusing compensation for the inhibition reaction step described by $v(s) = \frac{c}{K_M+s}$: SF-SD was investigated for different distributions of $s$ such as the Poisson distribution and the negative binomial distribution with burst size $b = 8, 50$. For computation, Jarnac [1] and R [2] were used.

## S3 Noise-enhanced concentration detector

We apply stochastic focusing compensation to incoherent feedforward gene regulatory networks that function as concentration detectors [3, 4], to enhance their detection amplitudes and sensitivities. Incoherent feedforward networks are known to function as concentration detectors [3, 4]. Consider a reaction process where a protein ($S_2$) is regulated by two different pathways: either directly by a transcription factor $X_0$ or indirectly via another factor $S_1$ as shown in Fig. S2a. The direct control activates the expression of $S_2$ while the indirect control inhibits it. Thus, the feedforward is called incoherent. When the concentration of $X_0$ is zero, $S_2$ is not expressed. As $X_0$ increases, $S_2$ increases (this region of $X_0$ will be named OFF→ON as shown in Fig. S2e): $S_2 \simeq \alpha(p_3/p_5)X_0$ for sufficiently small $X_0$, which means that in the log-log plot of $S_2$ vs. $X_0$, the slope is +1 (Fig. S2d Deterministic Case). When $X_0$ becomes larger than a thresh-hold point, it begins, however, to decrease and is eventually dominated by $S_2$'s inhibition (the region of $X_0$ will be named ON→OFF as shown in Fig. S2e) by following $S_2 \simeq \alpha p_2 p_3/p_1 p_4 p_5 X_0$. This means that the slope in the log-log plot is $-1$ (Fig. S2d Deterministic Case). Thus, one can detect a specific range of the concentration of $X_0$ by monitoring the concentration of $S_2$.

Now, consider stochastic effects on the incoherent feedforward network. Stochastic focusing compensation will be applied to enhance the detection amplitude and sensitivity. Based on the fact that $S_1$ inhibits the synthesis of $S_2$ hyperbolically, we can conclude that both **strong** stochastic focusing and de-focusing, due to stochastic focusing compensation, can appear in the ON→OFF region (refer to Fig. S1). Based on the fact that $X_0$ activates the synthesis of $S_2$ hyperbolically (Hill coefficient equal to one), we can achieve only **weak** stochastic focusing in the OFF→ON region (see the main manuscript Figure 2e and f). Although the stochastic effect via the activation pathway is weak, it will become useful to investigate for understanding how the effect can change depending on network topology.

We focus on the inhibition pathway and aim to increase the detection sensitivity in the ON→OFF region. For this aim, strong stochastic focusing is required to appear in the ON→OFF region, while minimizing the appearance of stochastic de-focusing in the region. For the case of hyperbolic inhibition, strong stochastic focusing was achieved for the value of $K_M \lesssim 0.1$ nM (Fig. S1). Thus, we need to find the terms corresponding to $K_M$ and set its value less than 0.1 nM. Since $v_3$ is expressed by

$$v_3 = \frac{\alpha p_3 X_0}{(1 + p_3 X_0) + p_4 X_0 S_1},$$

the Michaelis-Menten constant $K_M$ corresponds to $(1 + p_3 X_0)/p_4 X_0$ and will be set to less than 0.1 nM.

Thus, we obtain the lower bound of $X_0$:

$$X_0 > \frac{1}{0.1p_4 - p_3}.$$

In addition, $S_1$ should fluctuate between 1 and 10 nM for achieving strong stochastic focusing (refer to Fig. S1). Since the mean value of $S_1$ is equal to $p_1X_0/p_2$, this will be set between 1 and 10 nM, providing the range of $X_0$:

$$\frac{p_2}{p_1} < X_0 < 10\frac{p_2}{p_1}.$$

Thus, the expected range of the value of $X_0$ for the strong stochastic focusing becomes

$$\text{MAX}\left(\frac{1}{0.1p_4 - p_3}, \frac{p_2}{p_1}\right) < X_0 < 10\frac{p_2}{p_1},$$

where the function MAX chooses the larger value of its parameter arguments. For the stochastic focusing to appear in the ON→OFF region, the above $X_0$ region needs to be placed to the right side of the detection peak ($\sqrt{p_2/p_1p_4}$) but not too far away from the peak to minimize the appearance of strong stochastic de-focusing in the region:

$$\sqrt{\frac{p_2}{p_1p_4}} \simeq \text{MAX}\left(\frac{1}{0.1p_4 - p_3}, \frac{p_2}{p_1}\right) < X_0 < 10\frac{p_2}{p_1}, \tag{S4}$$

We assigned initial parameter values such that the inequality condition (S4) is not satisfied: The lower and upper bounds of $X_0$ were set to 11.1 and 10 nM, and the value of $X_0$ corresponding to the peak amplitude was to 1 nM. The detection properties did not improve (Fig. S2d and e), because strong stochastic focusing was not achieved. We tuned the parameters to satisfy the condition (S4): The lower and upper bounds of $X_0$ were set to 1 and 10 nM, and the value of $X_0$ corresponding to the peak amplitude was to 1 nM. Concentration detection was enhanced in the ON→OFF sensitivity and amplitude (Fig. S2c). The sensitivity (slope in the log-log scale) was increased 5 times and the amplitude 7 times due to the strong stochastic focusing (in this Supplementary Information, the distribution of $S_1$ was assumed to follow the Poisson distribution for Fig S2a and b but in the main manuscript the gamma distribution was also considered, which caused much larger detection amplification). However, the bandwidth stayed the same (arrows in Fig. S2c), which is related to the stochastic focusing compensation; stochastic de-focusing appears as $X_0$ decreases away from the region of stochastic focusing, resulting in reduced detection sensitivity and eventually preventing the detection bandwidth from decreasing.

To enhance the detection amplitude and sensitivity further, we used the curvature-covariance effect on mean reaction rates. Since the curvature of $v_3$ with respect to $S_1$ is positive, stochastic focusing becomes stronger with the increase in the variance of $S_1$. To increase the variance, we replace the upstream genetic

network of the $S_1$ expression as in Fig. S2b: $X_0$ up-regulates the expression of two identical cistrons of $S_1$. Each cistron is expressed with the same reaction rate as in the original network, but the translated $S_1$ degrades two times faster. Thus, the mean concentration of $S_1$ does not change but its fluctuation increases [5]. This further amplified the detection up to 9 times compared to the deterministic case (Fig. S2f), with a minor increase in the bandwidth.

We modified the original upstream network in a different way to increase the noise level of $S_1$. $X_0$ was allowed to fluctuate, while both the mean levels of $X_0$ and $S_1$ stayed the same. Although the variance of $S_1$ increased due to the noise originating from $X_0$, the detection amplitude was reduced (Fig. S2e). This was because we did not take into account the direct effect of the variance of $X_0$ on $v_3$ and the indirect effect of the covariance between $X_0$ and $S_1$, both of which contributed to the detection amplitude negatively. From Eq. (C1) the curvature-covariance correction term is given by

$$\frac{1}{2}\frac{\partial^2 v_3}{\partial X_0^2}\sigma_{X_0,X_0} + \frac{\partial^2 v_3}{\partial X_0 \partial S_1}\sigma_{X_0,S_1} + \frac{1}{2}\frac{\partial^2 v_3}{\partial S_1^2}\sigma_{S_1,S_1},$$

where the first term is negative because the curvature is negative with respect to $X_0$, and the third term is positive because the curvature is positive with respect to $S_1$. The second term was shown to be negative because $\frac{\partial^2 v_3}{\partial X_0 \partial S_1}$ was negative and the covariance was positive. Thus, due to the negative contribution of the first and second terms, the detection amplitude becomes smaller than the original case.

## S4 Mutual inhibition between two genes

When the mutual inhibition occurs non-cooperatively (Hill coefficient equal to 1), it is impossible for the system to show bistability in the deterministic case. Consider mutual inhibition between two species $S_1$ and $S_2$, where $S_1$ is synthesized with a rate $v_1 = p_1/(1 + S_2/K_{M_2})$ and degrades with a rate $v_2 = p_2 S_1$; $S_2$ is synthesized with a rate $v_3 = p_3/(1 + S_1/K_{M_1})$ and degrades with a rate $v_4 = p_4 S_2$. At steady state, $v_1$ is equal to $v_2$, i.e., $S_1$ is equal to $(p_1/p_2)/(1 + S_2/K_{M_2})$. By substituting this to $v_3(S_1)$, we obtain a net non-cooperative positive feedback:

$$v_3 = \frac{p_3\left(1 + \frac{S_2}{K_{M_2}}\right)}{\frac{p_1}{K_{M_1} p_2} + 1 + \frac{S_2}{K_{M_2}}}.$$

At steady state, $v_3$ is equal to $v_4$:

$$\frac{p_3\left(1 + \frac{S_2}{K_{M_2}}\right)}{\frac{p_1}{K_{M_1} p_2} + 1 + \frac{S_2}{K_{M_2}}} = p_4 S_2.$$

This equation has only one positive stable solution, resulting in a single stable steady state.

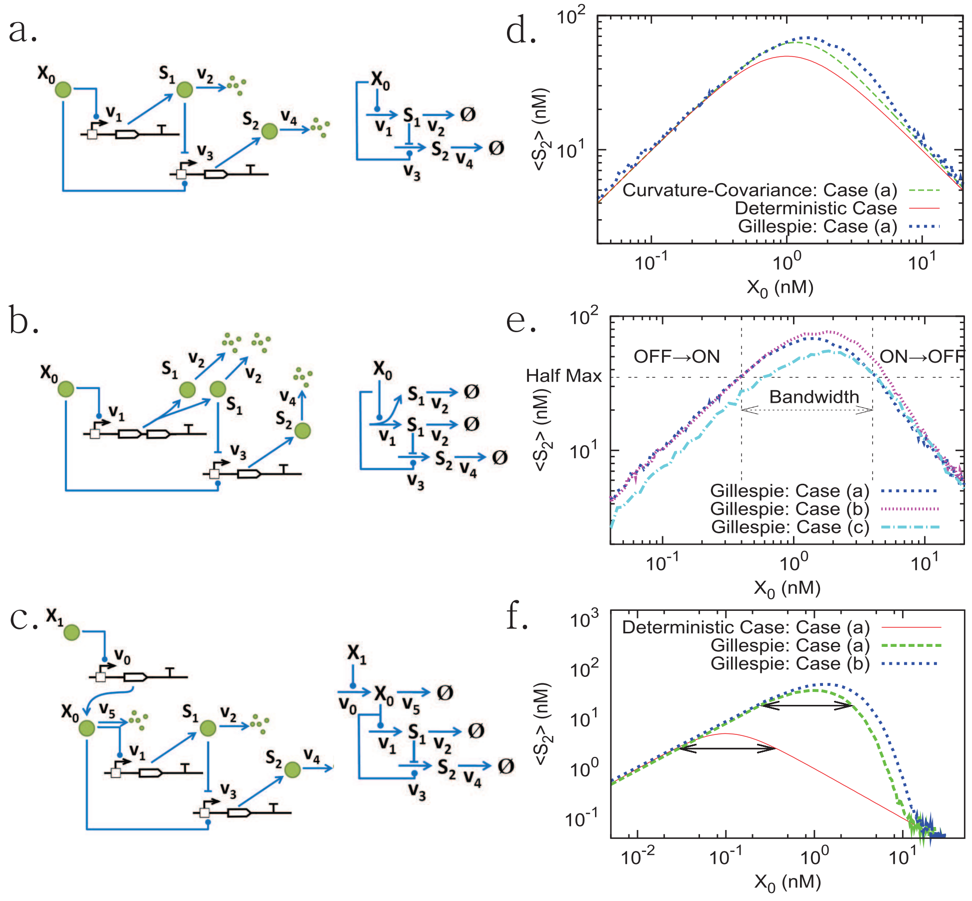


**Figure S2.** Noise-enhanced concentration detection: Three different incoherent feed-forward networks are considered. (a) A transcription factor $X_0$ up-regulates the expression of both $S_1$ and $S_2$, and $S_1$ down-regulates the expression of $S_2$. The concentration of $X_0$ is considered not changed (boundary species). Reaction rates: $v_1 = p_1X_0$, $v_2 = p_2S_1$, $v_3 = \frac{\alpha p_3/p_4}{S_1+(1+p_3X_0)/p_4X_0}$, and $v_4 = p_5S_2$. (b) $X_0$ up-regulates the expression of two identical cistrons expressing $S_1$. By using this set-up, the fluctuation in $S_1$ becomes larger than case (a), while the mean concentration of $S_1$ remains the same: All reactions are the same as case (a) except $v_2 = 2p_2S_1$. (c) $X_0$ is allowed to fluctuate and its synthesis is regulated by $X_1$ that is a boundary species. The synthesis of $X_0$ is modeled by $v_0 = p_0X_1$ and its degradation by $v_5 = p_6X_0$. (d,e) The system was not optimized for leveraging stochastic focusing compensation. For case (b), noise in $S_1$ became larger and caused the detection amplitude and ON→OFF sensitivity enhanced. For case (c), the introduction of another source of noise coming from $X_0$, however, decreased the detection amplitude. (f) The compensation was leveraged to improve detection amplitude and ON→OFF sensitivity. With the larger noise (case b), the detection amplitude was further enhanced. Stochastic simulations were performed by using the Gillespie stochastic simulation algorithm [6]. For the figures d and e: $p_0 = 100$ hr$^{-1}$, $p_1 = 100$ hr$^{-1}$, $p_2 = 100$ hr$^{-1}$, $p_3 = 0.01$ nM$^{-1}$, $p_4 = 1$ nM$^{-2}$, $p_5 = 10$ nM$^{-1}$hr$^{-1}$, $p_6 = 100$ hr$^{-1}$, and $\alpha = 10^5$ nM/hr. For the figure f: $p_1 = 100$ hr$^{-1}$, $p_2 = 100$ hr$^{-1}$, $p_3 = 0.01$ nM$^{-1}$, $p_4 = 100$ nM$^{-2}$, $p_5 = 10$ hr$^{-1}$, and $\alpha = 10^5$ nM/hr.

## S5 Noise-induced linear amplifier

Consider a reaction step described in Fig. 5a with the reaction rate given by the following Hill equation:

$$v(S) = \frac{v_{max} S^h}{K_M^h + S^h},$$

with $K_M = 25$ nM and $v_{max} = 1$ nM/hr. For a wide range of the Hill coefficient $h$, the distribution of the copy number of $S$ given by the negative binomial distribution – discrete version of the Gamma distribution – linearized the regulation as shown in Fig. S3.

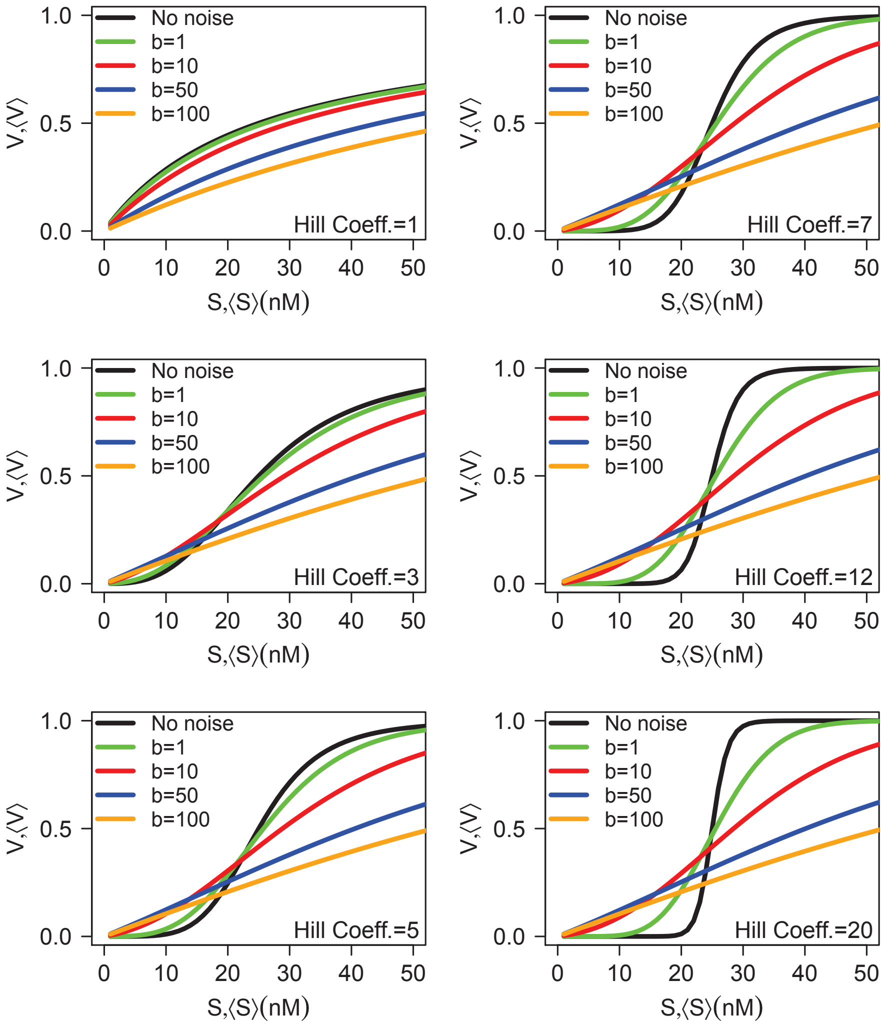


**Figure S3.** Noise-induced linearization for the Hill-type regulation, $v(S) = \frac{v_{max} S^h}{K_M^h + S^h}$: The Hill coefficients $h = 1, 3, 5, 7, 12, 20$ were used.

A different type of the Hill equation was also considered:

$$v(S) = \frac{v_{max} S^h}{K_M^h + K_1^{h/2} S^{h/2} + S^h},$$

with $K_M = 25$ nM, $K_1 = 25$ nM and $v_{max} = 1$ nM/hr. For a wide range of the Hill coefficient $h$, the noise in $S$ linearized the regulation as shown in Fig. S4.

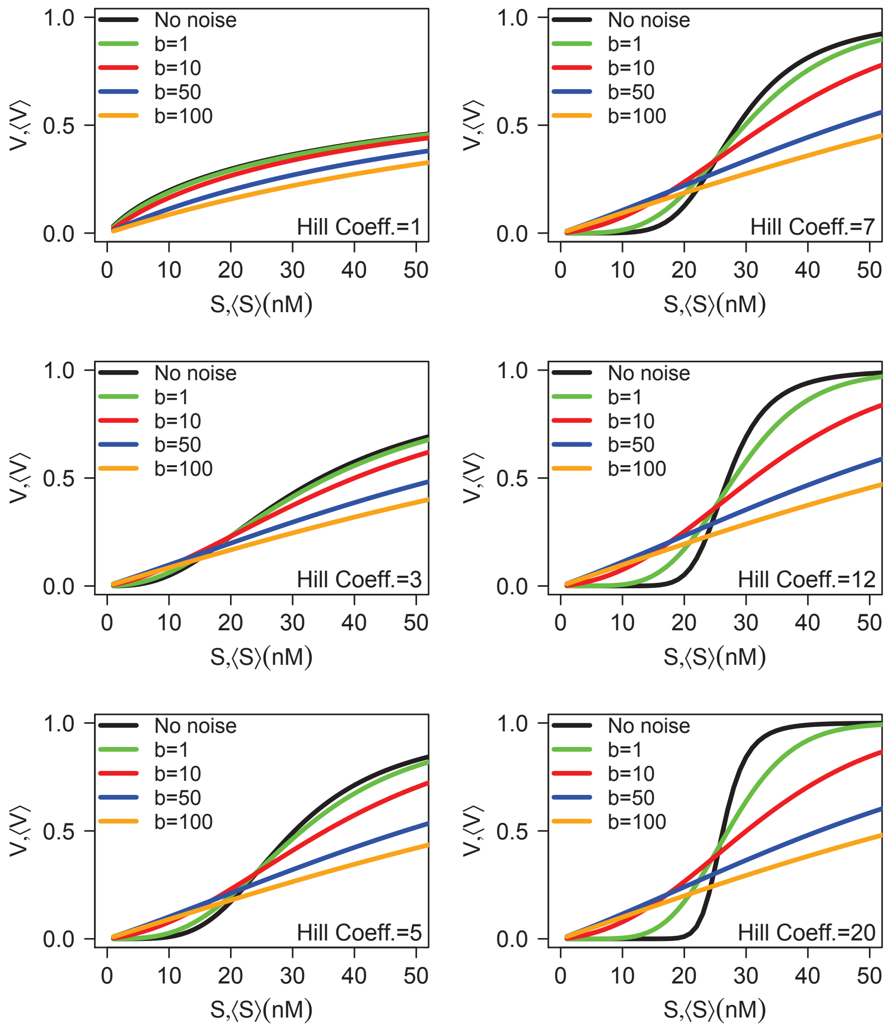


**Figure S4.** Noise-induced linearization for the Hill-type regulation, $v(S) = \frac{v_{max} S^h}{K_M^h + K_1^{h/2} S^{h/2} + S^h}$: The Hill coefficients $h = 1, 3, 5, 7, 12, 20$ were used.

To confirm this noise-induced linear amplification, stochastic simulations were performed for a three-gene cascade (Fig.5d) by using the Gillespie stochastic simulation algorithm [6], with transcription processes

included. The model is described as follows:

$$\xrightarrow{v_1} mRNA_1 \xrightarrow{\gamma_{m1} mRNA_1}$$
$$\xrightarrow{\alpha_{s1} mRNA_1} s_1 \xrightarrow{\gamma_{s1} s_1}$$
$$\xrightarrow{v_2(s_1)} mRNA_2 \xrightarrow{\gamma_{m2} mRNA_2}$$
$$\xrightarrow{\alpha_{s2} mRNA_2} s_2 \xrightarrow{\gamma_{s2} s_2}$$
$$\xrightarrow{v_3(s_2)} mRNA_3 \xrightarrow{\gamma_{m3} mRNA_3}$$
$$\xrightarrow{\alpha_{s3} mRNA_3} s_3 \xrightarrow{\gamma_{s3} s_3}$$

where $v_1$, $v_2$, and $v_3$ denote transcription rates:

$$\begin{aligned} v_1 &= 0.01 + vmax \frac{s_0^2}{K_{m0}^2 + s_0^2}, \\ v_2 &= 0.01 + vmax \frac{s_1^4}{K_{m1}^4 + s_1^4}, \\ v_3 &= 0.01 + vmax \frac{s_2^4}{K_{m2}^4 + s_2^4}, \end{aligned}$$

and the parameters are defined as:

$$K_{m0} = 10,\ K_{m1} = 25,\ K_{m2} = 25,\ \gamma_{m1} = 30,\ \gamma_{m2} = 30,\ \gamma_{m3} = 30,\ \gamma_{s1} = 2,\ \gamma_{s2} = 2,\ \gamma_{s3} = 2,$$

and

$$vmax = 100,\ \alpha_{s1} = 30,\ \alpha_{s2} = 30,\ \alpha_{s3} = 30,\ \text{for } b = 1,$$

$$vmax = 10,\ \alpha_{s1} = 300,\ \alpha_{s2} = 300,\ \alpha_{s3} = 300,\ \text{for } b = 10,$$

$$vmax = 2,\ \alpha_{s1} = 1500,\ \alpha_{s2} = 1500,\ \alpha_{s3} = 1500,\ \text{for } b = 50.$$

The value of $s_0$ was changed from 0 to 25.

## Software

All simulations and their numerical analysis were carried on custom codes, Systems Biology Workbench (www.sys-bio.org) [8, 9] and R [2].

## References


1. Sauro HM, Fell DA: **Jarnac: A system for interactive metabolic analysis**. In *Animating the Cellular Map: Proceedings of the 9th International Meeting on BioThermoKinetics*, Stellenbosch University Press 2000:221–228.

2. R Development Core Team: *R: A language and environment for statistical computing.* Vienna, Austria: R Foundation for Statistical Computing 2008.

3. Entus R, Aufderheide B, Sauro HM: **Design and implementation of three incoherent feed-forward motif based biological concentration sensors.** *Syst. Synth. Biol.* 2007, **1**:119–128.

4. Kaplan S, Bren A, Dekel E, Alon U: **The incoherent feed-forward loop can generate non-monotonic input functions for genes.** *Mol. Syst. Biol.* 2008, **4**(203):203.

5. Elf J, Ehrenberg M: **Fast evaluation of fluctuations in biochemical networks with the linear noise approximation.** *Genome Res.* 2003, **13**(11):2475–2484.

6. Gillespie DT: **Exact stochastic simulation of coupled chemical reactions.** *J. Phys. Chem.* 1977, **81**:2340–2361.

7. Paulsson J, Berg OG, Ehrenberg M: **Stochastic focusing: fluctuation-enhanced sensitivity of intracellular regulation.** *Proc. Natl. Acad. Sci. U. S. A.* 2000, **97**(13):7148–7153.

8. Sauro HM, Hucka M, Finney A, Wellock C, Bolouri H, Doyle J, Kitano H: **Next generation simulation tools: the Systems Biology Workbench and BioSPICE integration.** *OMICS* 2003, **7**(4):355–372.

9. Bergmann FT, Vallabhajosyula RR, Sauro HM: **Computational Tools for Modeling Protein Networks**. *Curr. Proteomics* 2006, **3**(3):181–197.
